# Supplementary material for: \AA ngstrom depth resolution with chemical specificity at the liquid-vapor interface
Source: arXiv:2209.15437 source file (2023-02-14)
Supplement: Supplementary file 1 [file Supp_Mat.pdf]

# Supplemental Material to "Ångstrom depth resolution with chemical specificity at the liquid-vapor interface"

R. Dupuy, J. Filser, C. Richter, T. Buttersack, F. Trinter, S. Gholami, R. Seidel, C. Nicolas, J. Bozek, D. Egger, H. Oberhofer, S. Thürmer, U. Hergenhahn, K. Reuter, B. Winter and H. Bluhm

## Contents

**1 Experimental details and data analysis** **2**
1.1 Gas-phase measurements . . . 2
1.2 Extraction of $\beta$ parameters . . . 2
1.3 Gas-phase $\beta$ values and as-measured liquid $\beta$ values . . . 4
1.4 Sensitivity limit of the measurements . . . 4

**2 Molecular dynamics simulations** **5**
2.1 Methods . . . 5
2.2 Force-field parameterization . . . 6
2.3 Bias potential . . . 9

**3 Validity of the $\beta$ linearity** **10**

## List of Figures

S1 O 1s gas-phase spectrum of PFPA. . . . 2
S2 Sketch of the experimental geometry. . . . 3
S3 C 1s PADs of 100 mM NaPFP solution. . . . 3
S4 O 1s spectrum and PAD of a NaPFP 100 mM solution. . . . 4
S5 Sample snapshot from MD simulation. . . . 6
S6 Vertical distributions relative to the instantaneous water surface in the MD simulation. . . . 7
S7 Torsional profiles of dihedrals in PFP for which force field parameters were fitted in this work. . . . 8
S8 Biased and unbiased vertical distributions in the MD simulation. . . . 9
S9 Vertical distributions between bulk and surface in the MD simulation. . . . 10
S10 Differential elastic-scattering cross sections and their effect on the anisotropy parameter . . . 11

# 1 Experimental details and data analysis

## 1.1 Gas-phase measurements

Gas-phase measurements of photoelectron angular distributions (PADs) were performed to serve as reference for the liquid-phase measurements. As mentioned in the main text, it is important to perform these measurements because we want to extract the reduction of anisotropy of the nascent PAD, i.e., the intrinsic photoemission angular distribution from the condensed-phase molecule, caused by elastic scattering. The nascent PAD in the liquid is assumed to correspond to the gas-phase PAD, which is an approximation, as the molecule is necessarily affected by the aqueous environment. Changes in orbital character or structural changes due to solvation can, in principle, affect the nascent PAD. Since we are probing core levels, orbital or electronic structure changes are considerably reduced as compared to, e.g., shallow valence orbitals. Intramolecular scattering, on the other hand, could conceivably be affected if the molecule undergoes significant conformational changes upon solvation, but we consider this unlikely and will make the hypothesis that this effect can be neglected. The fact that the observed trends are linear at the three eKEs in Fig. 2 of the main text hints at only a small influence of above effects, which would be much more pronounced closer to the threshold.

Gas-phase measurements were performed at the PLEIADES beamline under the same conditions as the liquid-phase measurements. The gas was introduced into the enclosure with the microjet through the catcher aperture, while the jet was not running. The C 1s gas-phase spectrum of PFPA has already been shown in Fig. 1 of the main text. In Fig. S1 we show the O 1s gas-phase spectrum of PFPA. Two distinct bands are observed, originating from a chemical shift of about 2 eV between the C-O-H (lower binding energy) and C=O (higher binding energy) groups.

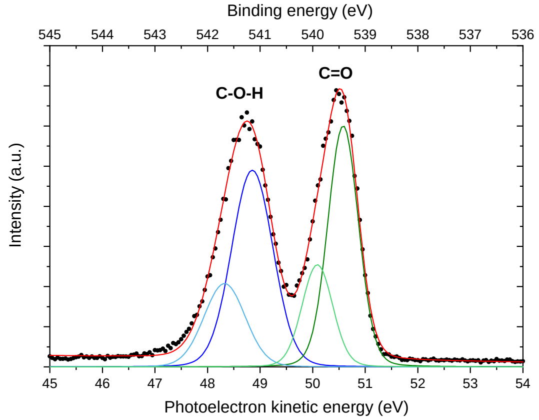


Figure S1: O 1s gas-phase spectrum of PFPA, measured at eKE $\sim$ 50 eV ($h\nu$ = 590 eV). Two distinct bands are labeled in the figure. Each band was fitted with two Gaussians to account for peak asymmetry, which do not have any physical meaning.

## 1.2 Extraction of $\beta$ parameters

The experimental geometry used for PAD measurements is sketched in fig. S2. PADs were measured by varying the angle of the linear polarization vector of the incident X-ray synchrotron beam with respect to the detection direction, effectively rotating the angular distribution. Spectra were recorded at angles between 0° and 90°. The procedure is similar to that described in previous papers [1, 2, 3].

Stability of the PE (photoelectron) signal is important for a correct assessment of the PAD, and, thus, measurements at 0° were frequently repeated during a measurement series as a stability check. Signal intensities are subsequently corrected for slight photon-flux variations at different polarization angles, which were measured using either a standard AXUV photodiode (at the PLEIADES beamline) or the mirror current on the first mirror (at the UE52_SGM beamline). These normalized intensities as a function of polarization angle are then fitted with the following formula:

$$f(\theta) = A\left(1 + \frac{\beta}{2}(3\cos^2(\theta + \theta_0) - 1)\right) \tag{1}$$

This equation is similar to Eq. 1 in the main text, except it includes a scaling term A and an offset term $\theta_0$ which accounts for a possible slight tilt of the apparatus, vertical beam misalignment, and a systematic difference between

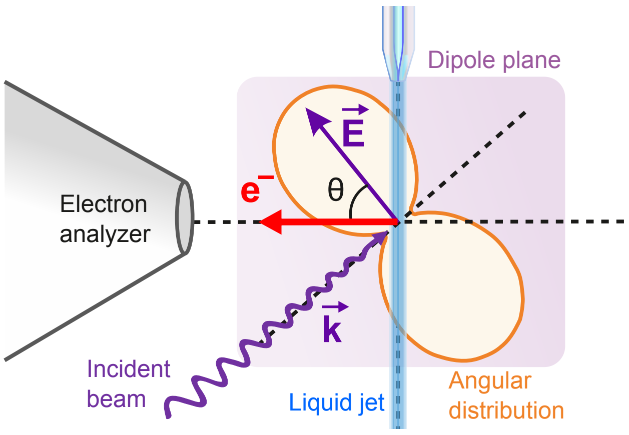


Figure S2: Sketch of the experimental geometry. The light propagation vector $\vec{k}$, detection direction, and liquid-jet propagation direction are all orthogonal, *i.e.*, the latter two comprise the dipole plane, defined as orthogonal to the light propagation direction. The direction of the light polarization vector $\vec{E}$ can be varied within the dipole plane between 0 and 90° with respect to the detection direction.

the nominal and actual polarization direction, e.g., due to a misalignment of the elliptically polarized undulator). In using Eq. (1), we assume that the synchrotron radiation is perfectly linearly polarized at any angle. An example of measured PADs is given in Fig. S3, with each panel corresponding to one distinguishable carbon peak of a 100 mM NaPFP solution measured at eKE ∼ 150 eV. The PADs were then fitted with Eq. (1).

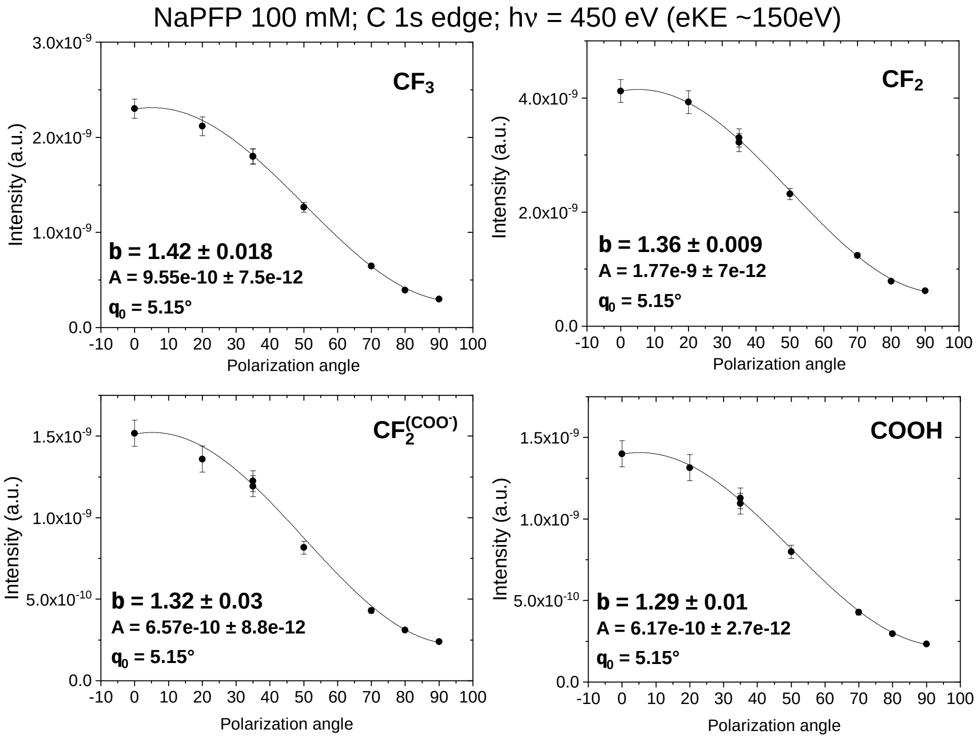


Figure S3: Measured photoelectron angular distributions (PADs) of the different distinguishable C 1s carbon peaks of a 100 mM NaPFP solution, at hν = 450 eV corresponding to eKE ∼ 150 eV. The PADs were fitted with Eq. (1), yielding the parameters indicated in each panel.

In the main text, in addition to the C 1s data, we also present $R_\beta$ values extracted from a measurement of the

O 1s band. In Fig. S4, we show the O 1s spectrum for the same 100 mM NaPFP solution and the extracted PAD. The spectrum was acquired in the same conditions as the C 1s spectrum of Fig. 1 of the main text, e.g, for a photon energy yielding eKE = 50 eV and at the magic angle.

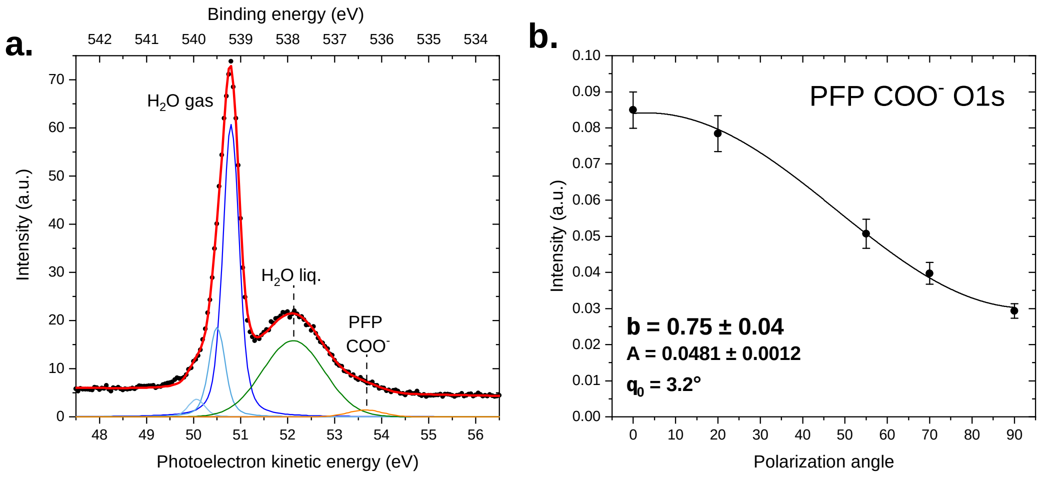


Figure S4: **a.** O 1s spectrum of a 100 mM NaPFP solution, measured at 590 eV photon energy (eKE ∼ 50 eV) at the magic angle. All components of the spectrum are labeled in the panel. **b.** Measured PAD of the $COO^-$ O 1s peak from panel a.

In the O 1s spectrum (Fig. S4a), the signature of the $COO^-$ oxygen atoms appears as a shoulder at the low-binding-energy side of the liquid-water peak. Fitting constraints (fixed widths and relative positions) were used to ensure a proper extraction of the $COO^-$ intensities, but the large overlap of the peaks adds to the uncertainty of the measurement. Note that the two oxygen atoms of the $COO^-$ group are equivalent here, contrary to the case of the COOH oxygen atoms of gas-phase PFPA presented in Fig. S1, which exhibits two distinct bands with different $\beta$ parameters, also tabulated below in Table S1. The difference of gas-phase $\beta$ value of the two non-equivalent COOH oxygen atoms can be attributed to a difference of intramolecular scattering. For a comparison to the liquid $COO^-$ oxygen atoms $\beta$ values, we used the gas-phase $\beta$ of the C=O peak. Scattering occurs mostly on nuclei, and, therefore, the nascent anisotropy of the $COO^-$ oxygen atoms PAD should be closer to that of the C=O oxygen peak PAD.

## 1.3 Gas-phase $\beta$ values and as-measured liquid $\beta$ values

The measured values of $\beta$ for gas-phase PFPA at different eKE are given in Table S1. Table S2 presents the as-measured $\beta$ values for the 100 mM NaPFP solution that were used for Figs. 2 and 3 of the main text. Table S3 lists the results for three repeated experiments performed on different days and on two different beamlines at eKE ∼ 150 eV. The $\beta$ values match within error bars of ±0.02.

Table S1: Extracted $\beta$ values for gas-phase PFPA at different eKEs.

| | PFPA C 1s | | | PFPA O 1s | |
|---|---|---|---|---|---|
| | $CF_3$ | $CF_2$ | COOH | C-O-H | O=C |
| eKE ∼ 50 eV | 1.01 ± 0.005 | 1.03 ± 0.007 | 1.28 ± 0.017 | 1.69 ± 0.004 | 1.59 ± 0.004 |
| eKE ∼ 150 eV | 1.66 ± 0.015 | 1.67 ± 0.027 | 1.73 ± 0.027 | | |
| eKE ∼ 350 eV | 1.79 ± 0.05 | 1.79 ± 0.05 | 1.82 ± 0.05 | | |

## 1.4 Sensitivity limit of the measurements

In the main text, the sensitivity limit of our measurements, in the sense of what is the smallest distance between two (classes of) atoms that can be separated by comparing their $R_\beta$ value, is discussed. The natural criterion for this distinction is that the error bars of two adjacent $R_\beta$ values should not overlap. The error bars of the as-measured $\beta$ values are determined from the fit result (see, e.g., Fig. S3). They typically vary between ±0.01 and ±0.04. After error propagation, this results in errors for $R_\beta$ between ±0.04 and ±0.06, as mentioned in the main text.

Table S2: Liquid-phase $\beta$ values before normalization for 100 mM NaPFP solution at different eKEs.

| | PFPA C 1s | | | | PFPA O 1s |
|---|---|---|---|---|---|
| | $CF_3$ | $CF_2$ | $CF_2^{(COO^-)}$ | $COO^-$ | $COO^-$ |
| eKE ∼ 50 eV | 0.82 ± 0.017 | 0.76 ± 0.014 | 0.69 ± 0.013 | 0.80 ± 0.013 | 0.92 ± 0.012 |
| eKE ∼ 150 eV | 1.43 ± 0.02 | 1.37 ± 0.01 | 1.32 ± 0.02 | 1.30 ± 0.01 | |
| eKE ∼ 350 eV | 1.75 ± 0.04 | 1.68 ± 0.05 | 1.60 ± 0.06 | 1.62 ± 0.05 | |

Table S3: $\beta$ values from three repeated measurements across different days and measurement campaigns. NaPFP 100 mM PADs were measured at a photon energy to yield eKE ∼ 150 eV at the C 1s edge. Experiment (1) was conducted at the PLEIADES beamline. Experiment (2) was conducted during the same beamtime, three days later, using a different batch of solution. Experiment (3) was conducted at the UE52_SGM beamline.

| | PFPA C 1s | | | |
|---|---|---|---|---|
| | $CF_3$ | $CF_2$ | $CF_2^{(COO^-)}$ | $COO^-$ |
| Experiment (1) | 1.44 ± 0.015 | 1.38 ± 0.01 | 1.32 ± 0.02 | 1.31 ± 0.02 |
| Experiment (2) | 1.42 ± 0.018 | 1.36 ± 0.009 | 1.32 ± 0.03 | 1.29 ± 0.01 |
| Experiment (3) | 1.42 ± 0.02 | 1.38 ± 0.015 | 1.32 ± 0.015 | 1.30 ± 0.018 |

Errors on the PE intensities, which are in turn carried over to errors on $\beta$ values, have several possible origins aside from statistical fluctuations: First in the experimental measurement and the associated normalization procedures, and then in the evaluation of peak areas by fitting. For the latter, errors can be introduced by systematic bias present in the chosen fit constraints. This is difficult to quantitatively evaluate, but 'hand-made' estimates showed us that changing the fit constraints had little effect on the relative difference of $\beta$ (within the error bars), while potentially introducing slight differences in the absolute values.

The most important source of experimental error is probably the change of alignment caused by slight variations in the jet position, which can hardly be avoided. This can be both caused by slow drifts over minutes or longer or abrupt position changes. Although this is partly accounted for by regularly checking the absolute count rate in the spectrum measured with vertical polarization and used as a reference, it remains most likely the most important source of error overall. In comparison, fluctuations of the photon flux and the associated detectors, of the order of 1% or less, are deemed negligible.

In order to get a better idea of the experimental reproducibility, we repeated a given experiment three times: Two measurements were done with three days of temporal distance and using a different batch of solution at the PLEIADES beamline, and a third one was carried out at the UE52_SGM beamline. The results are shown in Table S3 and show consistency within our error bars of the order of ±0.02.

# 2 Molecular dynamics simulations

## 2.1 Methods

A molecular dynamics (MD) simulation was conducted using the LAMMPS [4, 5, 6] package, version `29 Oct 2020`. The SPC/Fw [7] model for water was used. OPLS-AA force fields (FFs) were generated using the LigParGen [8, 9] tool, with the exception of some torsional parameters, see section 2.2. CM5 charges [10] were calculated using the CM5-calculator [11], from Hirshfeld [12] charges based on a density functional theory (DFT) calculation at the globally optimized geometry. CM5 charges of chemically equivalent atoms were averaged. The PBE0 [13] exchange-correlation (xc) functional was used. The DFT calculation was done with FHI-aims [14, 15, 16, 17, 18], using its *really tight* default basis sets with additional `for_aux hydro 5 g 6.0` functions for all elements to increase the accuracy of the hybrid DFT calculation. Relativistic effects were treated by the scalar zeroth order regular approximation (ZORA) [14]. Van-der-Waals interactions were treated by the non-local many-body dispersion (MBD-NL) model in a post-SCF (self-consistent field) correction [19]. The 'M' parameter set of Ref. [20] was used for the $Na^+$ ions.

The simulation cell had fixed lengths of 50 Å with periodic boundary conditions in $x$ and $y$ directions. In $z$ direction, the cell was 210 Å long and periodic boundary conditions were only formally applied for the particle-particle particle-mesh (PPPM) solver [22, 23], but corrected for to yield effectively open boundary conditions in that direction [5]. 8358 water molecules were placed in the cell, amounting to an approximately 100 Å thick slab. fftool [24] and packmol [25], version `20.2.2` were used in the creation of the water box. Aiming for a bulk concentration of 100 mM NaPFP, 15 PFP anions and 15 $Na^+$ cations were inserted into the middle of the water slab. Aiming

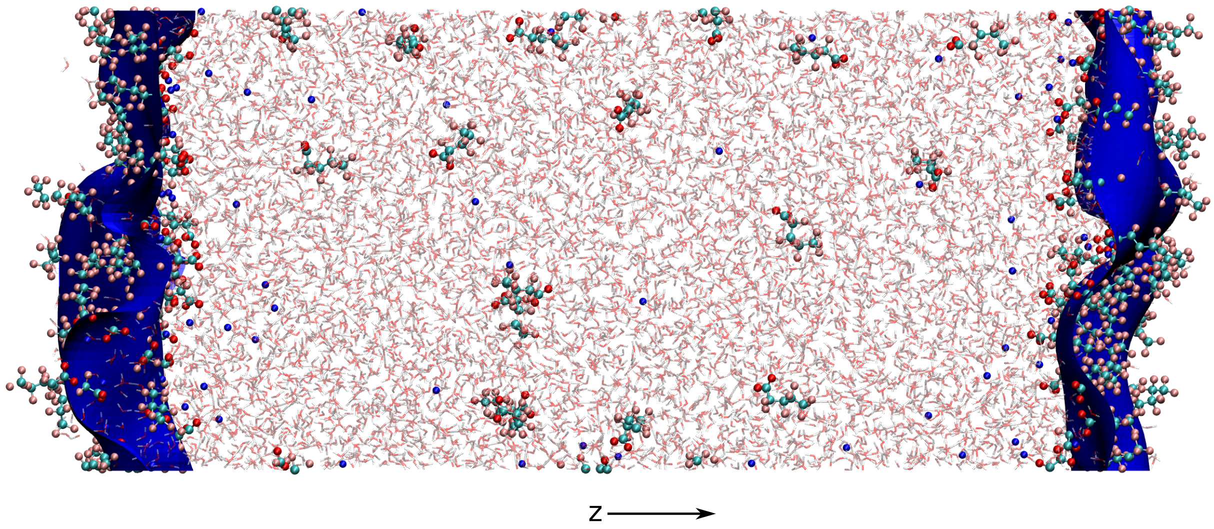


Figure S5: Snapshot from MD simulation. $Na^+$ shown in blue, C, O and F of PFP in teal, red and pink, respectively. Water molecules shown as transparent wedges. Instantaneous interfaces [21] shown as solid blue surfaces. One simulation cell is shown here. Periodic boundary conditions are applied in $x$ and $y$ directions to form a water slab.

for a surface coverage of $2.0 \cdot 10^{14}\,\mathrm{cm}^{-2}$, 50 such pairs were placed above the water slab, and 50 below it. This surface coverage corresponds to a rough estimate of the experimental surface coverage, based on surface tension measurements. One unit cell of the system after equilibration is shown in fig. S5.

Lennard-Jones walls were placed 5 Å above the lower and below the upper cell boundary to prevent molecules from leaving the simulation cell [5]. The used FFs underestimate the surface coverage to bulk concentration ratio of NaPFP. This was corrected by adjusting the chemical potential with a $z$-dependent bias potential as described in section 2.3.

The MD simulations were conducted in the $NVT$ ensemble by applying a Nosé-Hoover thermostat [26, 27] with fixed cell dimensions at 300 K. Drift of the water box as a whole in $z$ direction was prevented by subtracting the center-of-mass velocity from the velocities of all atoms in each time step and re-scaling the velocities to conserve kinetic energy [5]. Time steps of 1 fs were used. All systems were equilibrated for $2 \cdot 10^6$ time steps before running $2 \cdot 10^7$ time steps of production calculation. For evaluation, every 2000th MD step of the latter was used as a snapshot.

For the final analysis and comparison to our experimental data, distributions of the C and O atoms along the $z$ axis (i.e. the global surface normal) were determined relative to the instantaneous surface of the polar phase in the fashion of Ref. [21]. The polar phase was defined by Na and O atoms, including those of PFP. A coarse-graining length of $\xi = 3.16\,\text{Å}$ was chosen and the density isovalue for the interface was chosen to be half the maximum density in the bulk. The resulting instantaneous interface is illustrated in fig. S5, and the vertical distributions are shown in fig. S6.

## 2.2 Force-field parameterization

Torsional parameters for fluorinated molecules are not generally available in the OPLS-AA FF. For the F-CT-CT-F and CT-CT-CT-F torsions, we employ the parameters from Ref. [28]. For the remaining torsions, we developed our own set of parameters, retaining the functional form of OPLS-AA.

$$E(\theta) = \frac{1}{2}\left(V_1(1+\cos(\theta)) + V_2(1-\cos(2\theta)) + V_3(1+\cos(3\theta)) - V_4(1-\cos(4\theta))\right) \tag{2}$$

Here, $E$ is the energy contribution of a torsion, $\theta$ is the corresponding dihedral angle, and $V_1$ to $V_4$ are the to-be-determined parameters. In principle, the torsions without readily available parameters are: CT-CT-CT-CT, CT-

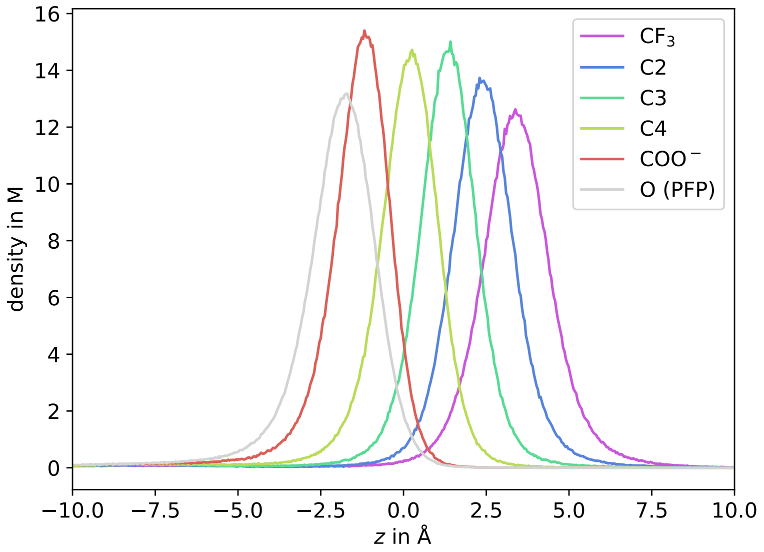


Figure S6: Vertical distributions of the C and O atoms of PFP relative to the instantaneous water surface in the MD simulation. Broader distributions towards the $CF_3$ end of the chain represent a higher vertical thermal mobility relative to the water surface.

CT-CT-C(=O), F-CT-CT-C(=O), F-CT-C=O, and CT-CT-C=O. However, CT-CT-C=O describes functionally the same torsion as F-CT-C=O, up to distortions in the tetrahedral coordination of the CT atom. The same can be said about CT-CT-CT-C(=O) and F-CT-CT-C(=O).

Therefore, three series of reference calculations were conducted in FHI-aims, using the same methods as described in the previous section. In each series, the corresponding dihedral angle (CT-CT-CT-CT, CT-CT-CT-C(=O), and CT-CT-C=O) was scanned in steps of 10°, starting at 180°. At each step, the molecular geometry was optimized, constraining the respective dihedral at the desired value. As an initial guess for geometry optimization, the optimized geometry from the previous step was used, with the dihedral adapted accordingly. Despite the molecule's symmetry, this scan was done over full 360°, to compensate for hysteresis in the geometries. The Atomic Simulation Environment ASE [29] was used for the constrained relaxation. Forces and energies for the relaxation were calculated with the *tight* default basis sets of FHI-aims with additional `for_aux hydro 5 g 6.0` functions. The energy of the optimized geometry was finally re-calculated using the basis described in the previous section.

OPLS-AA torsional parameters were fitted to the such obtained reference. In the present work, we are interested in equilibrium properties, but not in kinetics. Therefore, conformations with lower energy were given higher weights in the fitting than those with higher energy. Specifically, the following procedure was employed:

1. Conformation $i$, characterized by the respective dihedral angle $\theta_i$, with DFT reference energy $E_i^{\mathrm{ref}}$ was given a raw weight $w_i^{\mathrm{ref}} = \exp\left(-E_i^{\mathrm{ref}}/k_{\mathrm{B}}T\right)$ with the Boltzmann constant $k_{\mathrm{B}}$ and the temperature $T = 300\,\mathrm{K}$. For each series, the weights were then normalized according to $\widetilde{w}_i^{\mathrm{ref}} = w_i^{\mathrm{ref}} / \sum_j (w_j^{\mathrm{ref}})$. Each conformer was given an initial weight $\widetilde{w}_i = \widetilde{w}_i^{\mathrm{ref}}$.

2. Force-field parameters were calculated to minimize the error $p = \|\mathbf{E}^{\mathrm{ref}} - \mathbf{E}^{\mathrm{FF}}\|$ with the vectors $\mathbf{E}^{\mathrm{ref/FF}}$ containing the reference / force-field energies of all three series combined, weighted by $\widetilde{w}_i$. Force-field energies were calculated at the reference geometries. The weights of the CT-CT-C=O series were halved to account for symmetry. Since only energy differences are meaningful in classical FFs, one constant offset for each series was included in the fitting.

3. So far, this enforces that minima of the reference energy are reproduced well. However, additional minima of the force-field energy might exist elsewhere, which will also skew equilibrium distributions. Therefore, additional weights $w_i^{\mathrm{FF}}$ were calculated from the force-field energies and normalized in complete analogy to step 1. Each conformer was then given the averaged weight $\widetilde{w}_i = 1/2 \cdot (\widetilde{w}_i^{\mathrm{ref}} + \widetilde{w}_i^{\mathrm{FF}})$.

4. Steps 2 and 3 were repeated to self-consistency.

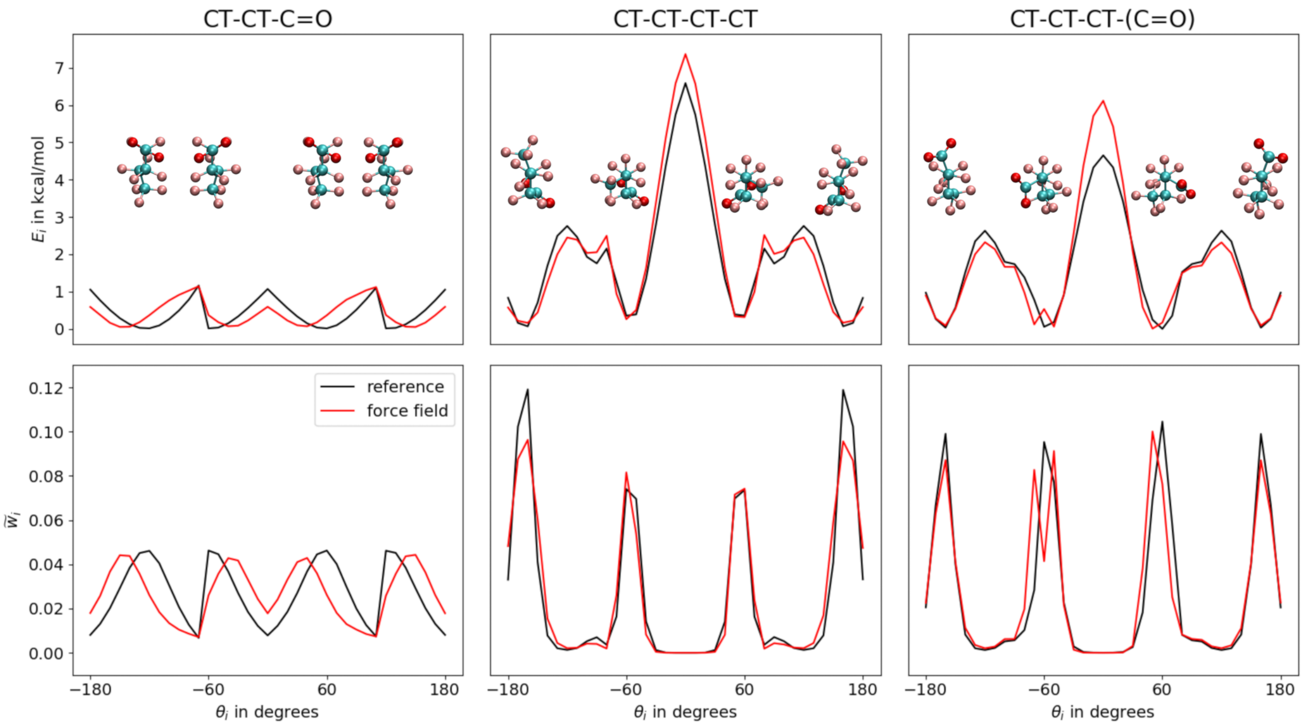


Figure S7: Energy profiles (top) and estimated thermal distributions (bottom) of the three torsions in PFP for which new OPLS-AA parameters were determined in this work (the first series scanned CT-CT-C=O in steps of 10°, but describing practically the same torsion by F-CT-C=O in the force-field energy turned out to yield a slightly smaller error). Geometries corresponding to the local minima of the reference energy shown as insets.

We introduce a second error function $p_2 = \|\widetilde{\mathbf{w}}^{\mathrm{ref}} - \widetilde{\mathbf{w}}^{\mathrm{FF}}\|$. Here, the vectors $\widetilde{\mathbf{w}}^{\mathrm{ref/FF}}$ contain $\widetilde{w}_i^{\mathrm{ref/FF}}$ of one of the three series. Since nuclear degrees of freedom except the three dihedral angles were optimized rather than thermodynamically sampled, $p_2$ gives only an estimate rather than an exact measure for the error in the thermal distributions.

The above procedure was re-iterated multiple times to avoid overfitting:

1. In the first fit, all terms of all 5 torsions were fitted freely, with the exception of the $\cos(\theta)$ and $\cos(3\theta)$ terms in the F-CT-C=O and CT-CT-C=O torsions, which would cancel due to symmetry. This produces large coefficients, indicating heavy overfitting; but it gives a lower bound on the errors $p_2$ that can be achieved within this model.

2. The highest of the coefficients was found ($V_1$ of the CT-CT-CT-C(=O) torsion) and its redundant counterpart ($V_1$ of F-CT-CT-C(=O)) identified. It was tested the removal of which of the two terms results in a smaller $\max(p_2)$ after re-fitting, with the maximum taken over the three series. From the resulting parameters, the highest one was found again and the procedure repeated, until no redundant pairs of parameters were left. This leaves us with 10 parameters: $V_2$ and $V_4$ of F-CT-C=O, and $V_1$ to $V_4$ of CT-CT-CT-CT and of CT-CT-CT-C(=O).

3. For each remaining term, it was tested if it can be removed without a significant increase in $p$ or $\max(p_2)$. This was the case for $V_2$ of CT-CT-CT-CT.

4. Lastly, $L_2$ regularization [30] was applied to reduce overfitting. The regularization strength was chosen as high as possible without significantly changing the thermal distributions between the *gauche* and (distorted) *anti* conformers of the two C-C-C-C torsions.

The final parameters are summarized in table S4, and the torsional profiles shown in fig. S7.

Table S4: OPLS-AA torsional parameters for PFP determined in this work, in kcal/mol.

| | F-CT-C=O | CT-CT-CT-CT | CT-CT-CT-C(=O) |
|---|---|---|---|
| $V_1$ | 0 | 4.981 | 5.453 |
| $V_2$ | -0.804 | 0 | -0.765 |
| $V_3$ | 0 | -2.062 | -0.662 |
| $V_4$ | 0.221 | -0.986 | -1.026 |

## 2.3 Bias potential

Running an MD simulation as described in section 2.1, but without the bias potential which will be discussed in this section leads to a significant portion of NaPFP diffusing from the water surface into bulk water. As seen in fig. S8(a), surface and bulk PFP can be clearly distinguished in the vertical distributions of the C atoms. For each C atom, the surface can be defined to begin at its concentration minimum.

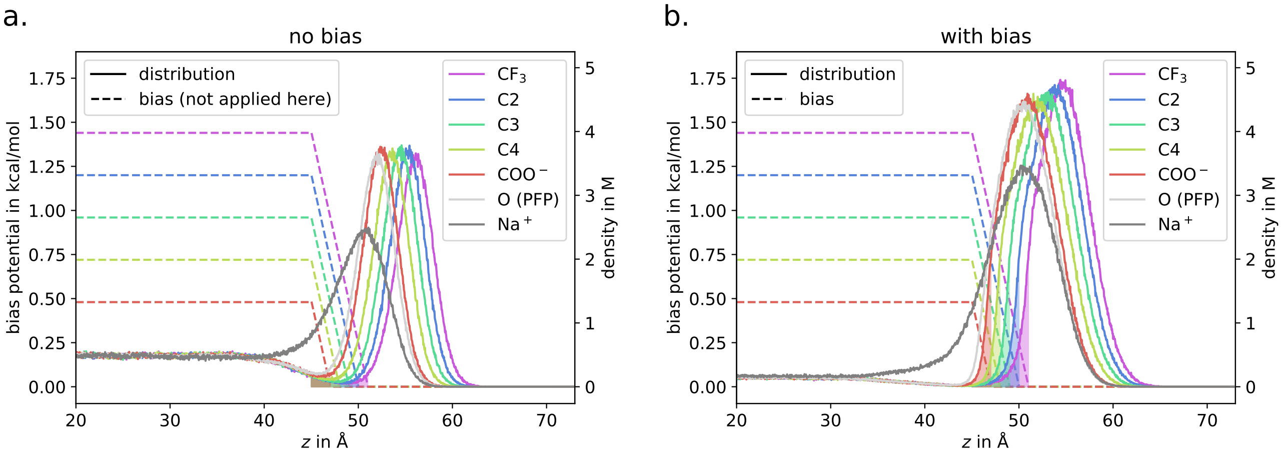


Figure S8: Vertical distributions of the different C atoms, as well as $Na^+$ and the O atoms of PFP with respect to the center of the water slab in the MD simulations. Data from upper and lower surface averaged. **a.** Without bias potential applied; bias shown only for reference. **b.** With bias potential. Shaded areas indicate the portion of C atoms which experience (or would experience, in the case of **a.**) a force from the bias potential.

To quantify the surface coverage, the peak of the $CF_3$ carbon atom, which shows the most pronounced minimum between bulk and surface, is integrated. All PFP anions which are not assigned to the surface in this way are assigned to the bulk. We further assume that the volume $V$ and surface area $A$ of our model system are exactly as in the initial geometry, i.e. $A = (50\,\text{Å})^2$ and $V = A \cdot 100\,\text{Å}$. With this information, we calculate a surface coverage of $1.08 \cdot 10^{14}\,\text{cm}^{-2}$, and a bulk concentration of 405 mM.

The error can be expressed in terms of an error in the chemical potential difference $\Delta\gamma$ between surface and bulk. The order of magnitude of this error can be estimated by assuming

$$\frac{\sigma(\text{Na}^+)\sigma(\text{PFP}^-)}{\rho(\text{Na}^+)\rho(\text{PFP}^-)} \sim \exp\left(-\frac{\Delta\gamma}{k_\text{B}T}\right) \tag{3}$$

with the surface coverages $\sigma$ and bulk concentrations $\rho$ of $Na^+$ and PFP. The values for PFP are obtained as described above, and we assume $\sigma(\text{Na}^+) = \sigma(\text{PFP}^-)$ and $\rho(\text{Na}^+) = \rho(\text{PFP}^-)$ for reasons of charge neutrality. With the values reported above, this leads to an estimated error in $\Delta\gamma$ of 2.4 kcal/mol.

With $Na^+$ known to be generally well soluble in water, we assume that the error in $\Delta\gamma$ originates from the PFP FF. We consequently apply a bias potential to the PFP anions, specifically to their C atoms. Ideally, we want the bias forces to act only in the transition region between bulk and surface, with constant bias potentials in both regions. Bias forces acting in the surface region would skew the property in which we are ultimately interested, i.e. the structure of the surfactant layer. In contrast, bias forces acting in the bulk would generate an unphyiscal

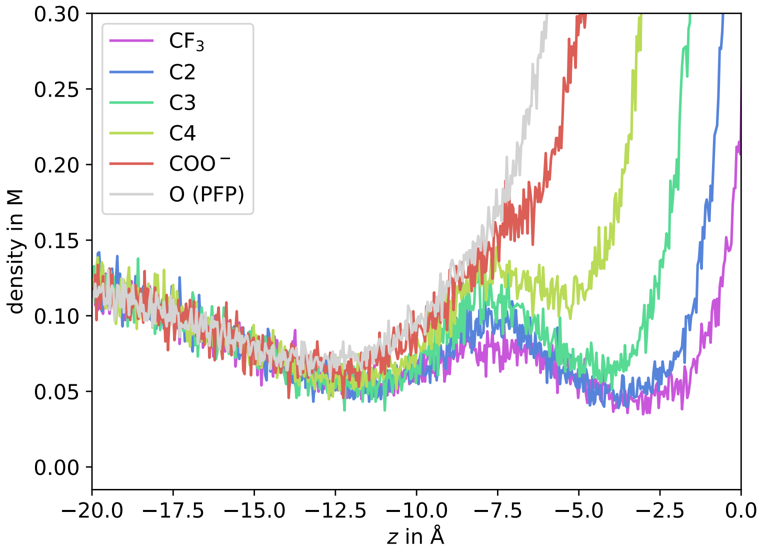


Figure S9: Vertical distributions of the C and O atoms of PFP relative to the instantaneous water surface with bias applied, in the transition region between bulk and surface.

sub-surface region with lower chemical potential than the bulk where PFP would accumulate, potentially perturbing the surfactant structure as well.

We choose a bias force which is constant [5] within the respective regions where it applies, and equal for all C atoms. For the carboxylic C atom, this force is applied in the region between 45 Å and 47 Å from the center of the water slab. For each further C atom along the chain, the upper limit was increased by 1 Å while the lower limit was kept fixed, as shown in fig. S8. The magnitude of the bias force was chosen such that the resulting potentials in the bulk sum up to the desired correction to $\Delta\gamma$. By systematic testing we find that the bias actually needs to be higher than the estimated 2.4 kcal/mol. At 4.8 kcal/mol, we achieve $\sigma(\mathrm{PFP}^-) = 1.96 \cdot 10^{14}\,\mathrm{cm}^{-2}$.

This results in an acceptable compromise between keeping the surface layer free from bias forces and preventing the formation of an unphysical sub-surface layer. Only 6.1 % of the $CF_3$ carbons in the surface layer actively experience the bias force, and the fraction is smaller for the other C atoms. On the other hand, a fluctuation in the distributions relative to the instantaneous water surface is observed below the surface layer, but it is small as seen in fig. S9.

## 3 Validity of the $\beta$ linearity

Equation 2 in the main text was derived from an analytical approximation of the differential scattering cross section (DCS) for elastic scattering by a Gaussian. This implies a number of limitations. Realistic DCS are more complex and for electron energies below 100 eV include a non-negligible backscattering component. As pointed out by Schild et al. [31], the convolution formula used here is only one-dimensional, whereas it would be more correct to use a two-dimensional convolution in spherical coordinates. To test the influence on the behavior of the scattered $\beta^*$ relative to the initial $\beta$, we numerically computed the $n$-fold convolution of an initial PAD with more realistic DCS. Only calculated DCS are used here, as the available experimental DCS, e.g. for gas phase water [32], do not measure the forward scattering component (close to 0°) which is in fact the most intense component by far. DCS curves for electron energies of 100 and 400 eV were extracted from the NIST electron elastic-scattering cross-sections database [33] using a model of water consisting of simply elemental oxygen and hydrogen. For comparison, the DCS calculated by Schild et al. [31] for a 7-water cluster model is shown, which was assumed by the authors to converge sufficiently towards bulk water behavior. These DCS are plotted in Fig. S10a. We also computed the 2D convolution of the PAD with the simple Gaussian DCS, using the formula given in Ref. [31].

The resulting $\beta^*$ as a function of the number of elastic scattering events $n$ is displayed in Fig. S10b. All curves were fitted using Eq. 2 from the main text. One can observe that all one-dimensional convolutions are perfectly fitted by Eq. 1, with only the effective value of $\phi$ changing. This formula seems to be valid no matter what the

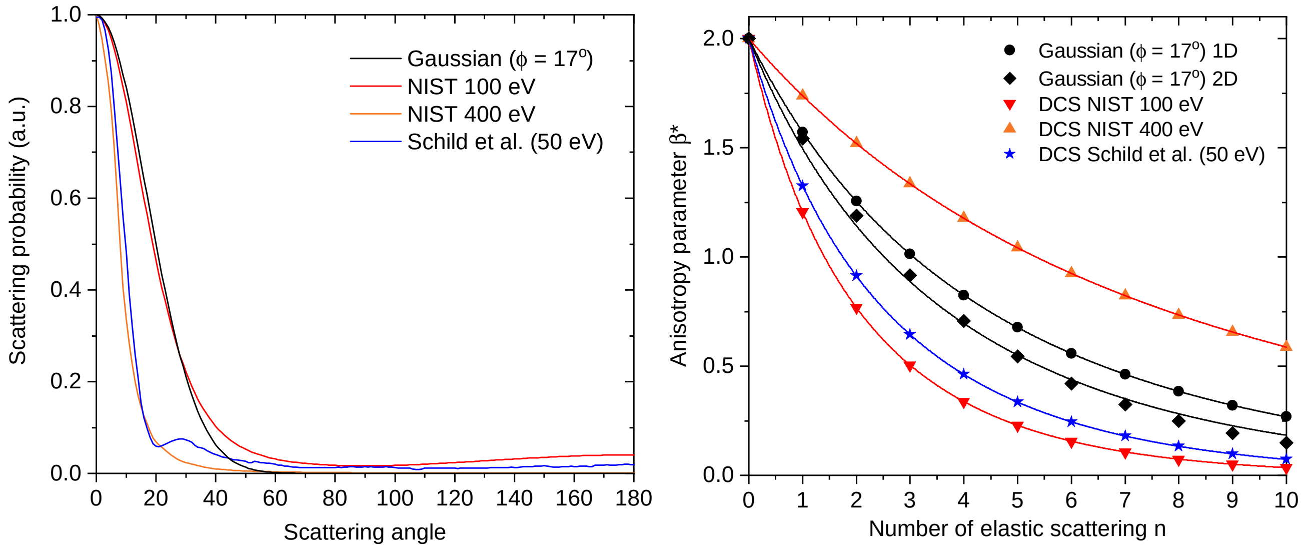


Figure S10: **a.** Examplary differential cross sections for elastic scattering, which were used to compute the data from panel b. References are given in the text. **b.** Computed anisotropy parameter $\beta^*$ of the distribution obtained after $n$-fold convolutions of various DCS with an initial PAD with $\beta = 2$.

exact shape of the DCS is. For the two-dimensional convolution, some discrepancies can be observed, but the equation can still reproduce fairly well the curve, with a slightly different effective $\phi$ than the one of the initial Gaussian. Schild et al. [31] also pointed out the potential importance of surface effects in the simulation of angular distributions. The surface, however, would not influence the linearity of the $\beta$ scale with depth.

In conclusion, linearity is always expected for low-$n$ regimes no matter what the shape of the DCS is. Only the regime of validity of the low-$n$ approximation changes. Since the appropriate DCS for our experiments is not easily accessible and other effects may come into play, we refrain from interpreting the absolute value of the slope.

# References


[1] R. Dupuy *et al.*, Phys. Chem. Chem. Phys. **24**, 4796 (2022).

[2] T. Lewis *et al.*, J. Phys. Chem. C **123**, 8160 (2019).

[3] S. Thürmer *et al.*, Phys. Rev. Lett. **111**, 173005 (2013).

[4] S. Plimpton, J. Comput. Phys. **117**, 1 (1995).

[5] S. Plimpton, A. Kohlmeyer, A. Thompson, S. Moore, and R. Berger, LAMMPS Stable release 29 September 2021 (stable_29Sep2021_update3). Zenodo., 2020.

[6] A. P. Thompson *et al.*, Comput. Phys. Commun. **271**, 108171 (2022).

[7] Y. Wu, H. L. Tepper, and G. A. Voth, J. Chem. Phys. **124**, 024503 (2006).

[8] W. L. Jorgensen and J. Tirado-Rives, Proc. Natl. Acad. Sci. U.S.A. **102**, 6665 (2005).

[9] L. S. Dodda, I. Cabeza de Vaca, J. Tirado-Rives, and W. L. Jorgensen, Nucleic Acids Res. **45**, W331 (2017).

[10] A. V. Marenich, S. V. Jerome, C. J. Cramer, and D. G. Truhlar, J. Chem. Theory Comput. **8**, 527 (2012).

[11] P. Melix, patrickmelix/cm5-calculator: First Production Release (v1.0), 2019.

[12] F. L. Hirshfeld, Theor. Chim. Acta **44**, 129 (1977).

[13] C. Adamo and V. Barone, J. Chem. Phys. **110**, 6158 (1999).

[14] V. Blum *et al.*, Comput. Phys. Commun. **180**, 2175 (2009).

[15] X. Ren *et al.*, New J. Phys. **14**, 053020 (2012).

[16] V. W. Yu *et al.*, Comput. Phys. Commun. **222**, 267 (2018).

[17] V. Havu, V. Blum, P. Havu, and M. Scheffler, J. Comput. Phys. **228**, 8367 (2009).

[18] A. C. Ihrig *et al.*, New J. Phys. **17**, 093020 (2015).

[19] J. Hermann and A. Tkatchenko, Phys. Rev. Lett. **124**, 146401 (2020).

[20] M. M. Reif and P. H. Hünenberger, J. Chem. Phys. **134**, 144104 (2011).

[21] Z. Liu, T. Stecher, H. Oberhofer, K. Reuter, and C. Scheurer, Mol. Phys. **116**, 3409 (2018).

[22] R. W. Hockney and J. W. Eastwood, *Computer Simulation Using Particles* (Routledge; Special Student ed., 1988).

[23] R. E. Isele-Holder, W. Mitchell, and A. E. Ismail, J. Chem. Phys. **137**, 174107 (2012).

[24] A. Padua, agiliopadua/fftool: Update (v1.1). Zenodo., 2019.

[25] L. Martínez, R. Andrade, E. G. Birgin, and J. M. Martínez, J. Comput. Chem. **30**, 2157 (2009).

[26] S. Nosé, J. Chem. Phys. **81**, 511 (1984).

[27] W. G. Hoover, Phys. Rev. A **31**, 1695 (1985).

[28] E. K. Watkins and W. L. Jorgensen, J. Phys. Chem. A **105**, 4118 (2001).

[29] A. H. Larsen *et al.*, J. Phys.: Condens. Matter **29**, 273002 (2017).

[30] A. Y. Ng, Feature selection, L1 vs. L2 regularization, and rotational invariance, in *Proceedings of the Twenty-First International Conference on Machine Learning*, ICML '04, p. 78, New York, NY, USA, 2004, Association for Computing Machinery.

[31] A. Schild, M. Peper, C. Perry, D. Rattenbacher, and H. J. Wörner, J. Phys. Chem. Lett. **11**, 1128 (2020).

[32] M. A. Khakoo *et al.*, Phys. Rev. A **78**, 052710 (2008).

[33] A. Jablonski, F. Salvat, C. J. Powell, and A. Y. Lee, *NIST Electron Elastic-Scattering Cross-Section Database Version 4.0, NIST Standard Reference Database Number 64* (National Institute of Standards and Technology, Gaithersburg, MD, 2016).
